# Supplementary material for: Representative Image Feature Extraction via Contrastive Learning Pretraining for Chest X-ray Report Generation
Source: arXiv:2209.01604 source file (2023-01-08)
Supplement: Supplementary file 1 [file appendix_B.tex]

\begin{table}[h]
\centering
\begin{tabular}{crrr}
\hline
\multicolumn{1}{l}{} & \multicolumn{1}{c}{Precision} & \multicolumn{1}{c}{Recall} & \multicolumn{1}{c}{F1} \\ 
\hline
AE                   & 0.451                         & 0.511                      & 0.480                  \\
SimCLR               & 0.480                         & 0.503                      & 0.490                  \\
\hline
\end{tabular}
\caption{Quantitative comparison of different encoder and decoder test on the IU X-Ray dataset. We evaluate the framework performance by matching the Medical Subject Headings (MeSH) tag of the generated and ground truth reports.}
\label{Table:encoder_F1}
\end{table}

Keywords are essential when evaluating medical reports since n-gram based evaluation might ignore the pivotal diagnoses when a sentence matches unimportant words well. For example, ``There is no pleural effusion'' and ``There is pleural effusion'' has opposite meaning while their scoring remains high in traditional metrics.  Moreover, we observed that most reports include clear and short sentences that describe objective diagnostic findings. 

Therefore, in this section, we evaluate our models' performance by matching the Medical Subject Headings (MeSH) tag of the generated and ground truth reports with the F1 score. First, we extract the Mesh tags of the sentences in the ground truths and the predictions. Then, we calculate the Precision, Recall, and F1 score of each sample. Finally, we obtain the results by taking the average of Precision, Recall, and F1 score of all samples respectively.

From Table \ref{Table:encoder_F1}, the F1 score shows that the SimCLR pretraining has a better performance than the AutoEncoder pretraining. Furthermore, we can observe that the SimCLR framework has higher precision than the AE framework, meaning that the SimCLR framework is more conservative when making predictions.
